# Supplementary material for: Cost-Efficient and Robust On-Demand Video Transcoding Using Heterogeneous Cloud Services
Source: arXiv:1711.01008 source file (2017-11-03)
Supplement: Supplementary file 1 [file appendix.tex]

\section{Table of Notations}\label{apdx:tbl}
\begin{table}[htbp]\caption{Description of symbols used in the paper}
\begin{center}% used the environment to augment the vertical space
% between the caption and the table
\begin{tabular}{r c p{10cm} }
\toprule
$G_{ij}$ & $\triangleq$ & GOP number $j$ in Video stream $i$\\
$U_i$ & $\triangleq$ & The utility value of GOP $i$\\
$\delta_{ij}$ & $\triangleq$ & The relative deadline of GOP number $j$ in Video stream $i$\\
$\Delta_{ij}$ & $\triangleq$ & The absolute deadline of GOP number $j$ in Video stream $i$\\  
$\psi_i$ & $\triangleq$ & the presentation start time of the video stream $i$\\
$VM_m$ & $\triangleq$ & Virtual Machine type $m$\\
$\tau^m_{ij}$ & $\triangleq$ & The estimated execution times of $G_{ij}$ on $VM_m$\\
$t_r$ & $\triangleq$ & The remaining estimated execution time of the currently executing task on a VM\\
$t_c$  & $\triangleq$ & Current time\\
$\varphi^m_n$ & $\triangleq$ & The estimated \emph{task completion time} of $G_n$ on $VM_m$\\
$\alpha$ & $\triangleq$ & The lower bound threshold for the deadline miss rate of GOPs\\  
$\beta$ & $\triangleq$ & upper bound threshold for the deadline miss rate of GOPs\\
$\gamma_{t}$ & $\triangleq$ & The deadline miss rate at any given time $t$\\
$r$ & $\triangleq$ & Streaming request arrival rate\\
$S_i$ & $\triangleq$ &  The suitability of VM type $i$ for a given GOP\\  
$T_i$ & $\triangleq$ & The performance of VM type $i$ for a given GOP\\
$C_i$ & $\triangleq$ & The cost of VM type $i$ for a given GOP\\  
$k$ & $\triangleq$ & A constant value\\
$\sigma_i$ & $\triangleq$ & Deadline miss rate for each GOP type $i$\\
$\phi_i$ & $\triangleq$ & Ratio of each GOP type $i$ in the batch queue \\
$\omega_i$ & $\triangleq$ & The demand for each VM type $i$  \\  
$\eta$ & $\triangleq$ & Degree of heterogeneity\\
$\rho_i$ & $\triangleq$ & The utilization of $VM_i$\\
$p_i$  & $\triangleq$ & Ratio of VM type $i$ of the total number of VMs\\
$N$  & $\triangleq$ & The total number of VMs\\
\bottomrule
\end{tabular}
\end{center}
\label{tab:TableOfNotationForMyResearch}
\end{table}

\section{Further Performance Evaluations of CVS2}\label{apdx:exp}
In Figure~\ref{fig:tpds_vs_ccgrid_m4}, we compared the QoS satisfaction (in terms of minimizing startup delay and deadline miss rate) of our proposed heterogeneous VM provisioning and scheduling methods against dynamic homogeneous VM provisioning and SDF scheduling method introduced in~\cite{pre_3}. 

In the first experiment, we consider General-Purpose VM type for homogeneous VM provisioning. As we can observe in Figure~\ref{fig:tpds_ccgrid_m4_cost}, homogeneous VM provisioning marginally reduces the incurred cost at the expense of a significantly lower QoS satisfaction (\ie higher startup delay and deadline miss rate, as shown in Figure~\ref{fig:tpds_ccgrid_m4_stt} and~\ref{fig:tpds_ccgrid_m4_dmr}.

\begin{figure*}[htbp]
\centering{
\subfigure[Comparison of average startup delay]
{\includegraphics[width=0.31\textwidth]{tpds_vs_ccgrid/het_vs_m4/stt}\label{fig:tpds_ccgrid_m4_stt}}
\subfigure[Comparison of average deadline miss rate]
{\includegraphics[width=0.31\textwidth]{tpds_vs_ccgrid/het_vs_m4/dmr}\label{fig:tpds_ccgrid_m4_dmr}}
\subfigure[Comparison of average cost]
{\includegraphics[width=0.31\textwidth]{tpds_vs_ccgrid/het_vs_m4/cost}\label{fig:tpds_ccgrid_m4_cost}}
\caption{Performance comparison under heterogeneous and homogeneous dynamic methods with \texttt{m4.large}. Subfigure (a) illustrates the average startup delay, (b) shows the average deadline miss rate, and (c) demonstrates the incurred cost under heterogeneous and homogeneous dynamic methods.}
\label{fig:tpds_vs_ccgrid_m4}}
\end{figure*}

\begin{figure*}[htbp]
\centering{
\subfigure[Comparison of average startup delay]
{\includegraphics[width=0.31\textwidth]{tpds_vs_ccgrid/het_vs_r3/stt}\label{fig:tpds_ccgrid_r3_stt}}
\subfigure[Comparison of average deadline miss rate]
{\includegraphics[width=0.31\textwidth]{tpds_vs_ccgrid/het_vs_r3/dmr}\label{fig:tpds_ccgrid_r3_dmr}}
\subfigure[Comparison of average cost]
{\includegraphics[width=0.31\textwidth]{tpds_vs_ccgrid/het_vs_r3/cost}\label{fig:tpds_ccgrid_r3_cost}}
\caption{Performance comparison under heterogeneous and homogeneous dynamic methods with \texttt{r3.xlarge}. Subfigure (a) illustrates the average startup delay, (b) shows the average deadline miss rate, and (c) demonstrates the incurred cost under heterogeneous and homogeneous dynamic methods.}
\label{fig:tpds_vs_ccgrid_r3}}
\end{figure*}

\begin{figure*}[htbp]
\centering{
\subfigure[Comparison of average startup delay]
{\includegraphics[width=0.31\textwidth]{tpds_vs_ccgrid/het_vs_g2/stt}\label{fig:tpds_ccgrid_g2_stt}}
\subfigure[Comparison of average deadline miss rate]
{\includegraphics[width=0.31\textwidth]{tpds_vs_ccgrid/het_vs_g2/dmr}\label{fig:tpds_ccgrid_g2_dmr}}
\subfigure[Comparison of average cost]
{\includegraphics[width=0.31\textwidth]{tpds_vs_ccgrid/het_vs_g2/cost}\label{fig:tpds_ccgrid_g2_cost}}
\caption{Performance comparison under heterogeneous and homogeneous dynamic methods with \texttt{g2.2xlarge}. Subfigure (a) illustrates the average startup delay, (b) shows the average deadline miss rate, and (c) demonstrates the incurred cost under heterogeneous and homogeneous dynamic methods.}
\label{fig:tpds_vs_ccgrid_g2}}
\end{figure*}

We also evaluated the performance and cost of dynamic homogeneous method when Memory-Optimized and GPU VM types are utilized. The results, shown in Figures~\ref{fig:tpds_vs_ccgrid_r3} and~\ref{fig:tpds_vs_ccgrid_g2} respectively, indicate that although the QoS satisfaction resulted from the homogeneous system is similar to the heterogeneous system (see Figures~\ref{fig:tpds_ccgrid_r3_stt}, \ref{fig:tpds_ccgrid_r3_dmr}, \ref{fig:tpds_ccgrid_g2_stt}, and \ref{fig:tpds_ccgrid_g2_dmr}), the incurred cost of homogeneous system has remarkably increased (see Figures~\ref{fig:tpds_ccgrid_r3_cost} and~\ref{fig:tpds_ccgrid_g2_cost}). 

The experiment results indicate that using heterogeneous VM types to process video transcoding tasks is effective in the sense it can provide the same QoS satisfaction while incurring a significantly lower incurred cost to the video stream provider.
